# Supplementary material for: Elucidating the local atomic and electronic structure of amorphous oxidized superconducting niobium films
Source: arXiv:2111.11590 source file (2021-11-23)
Supplement: Supplementary file 1 [file Nb_Structure_Exp_Th-SI.pdf]

# Supplementary Information for Elucidating the local atomic and electronic structure of oxidized superconducting niobium films

Thomas F. Harrelson,[1,2] Evan Sheridan,[1,2,3] Ellis Kennedy,[4] John Vinson,[5] Alpha T. N'Diaye,[6] M. Virginia P. Altoé,[2] Irfan Siddiqi,[1,7] Adam Schwartzberg,[2] D. Frank Ogletree,[2] Mary C. Scott,[4,8] and Sinéad M. Griffin[1,2]
[1)] *Materials Science Division, Lawrence Berkeley National Laboratory, Berkeley, CA 94720, USA*
[2)] *Molecular Foundry, Lawrence Berkeley National Laboratory, Berkeley, CA 94720, USA*
[3)] *Theory and Simulation of Condensed Matter, Department of Physics, King's College London, The Strand, London WC2R 2LS, UK.*
[4)] *Department of Materials Science and Engineering, University of California, Berkeley, CA 94720, USA*
[5)] *Material Measurement Laboratory, National Institute of Standards and Technology, Gaithersburg, MD 20899, USA*
[6)] *Advanced Light Source, Lawrence Berkeley National Laboratory, Berkeley, CA 94720, USA*
[7)] *Department of Physics, University of California, Berkeley, CA 94720, USA*
[8)] *NCEM, Molecular Foundry, Lawrence Berkeley National Laboratory, Berkeley, CA 94720, USA*

## I. FLUCTUATION ELECTRON MICROSCOPY

A full description of our FEM methodology applied to amorphous films is given in Ref.[1] In general, FEM data collection in a scanning transmission electron microscope consists of rastering a small focused probe over a sample, and collecting a series of nanodiffraction patterns.[2] Our FEM experiments were carried out using an FEI TitanX with an acceleration voltage of 200 kV. We set the third condenser lens current such that the convergence angle was 0.51 mrad, giving a measured 2.2 nm diameter probe and a 15.5 pA probe current. A beam stop was used to cover the central beam. We used an Orius CCD system for image collection with an exposure time of 0.3 s and a camera length of 300 mm. Our images were binned by a factor of four resulting in a final size of 512 × 512 pixels. All diffraction patterns for this set of experiments were taken with the same imaging conditions to account for possible effects of microscope misalignment across all patterns. Because the Nb-O film is extremely thin, (Fig. S1(a)), we took six small datasets and averaged them, to avoid contributions from other components of the device. Figure S1(b) illustrates the six regions from which the FEM scans were collected from the sample. Figure S1(b) is the resulting spatial variance obtained from radial integration of the the FEM speckle pattern for each of the regions in Figure S1(a).

FEM preprocessing consisted of correction for elliptical distortion following the prodocal outlined by Gammer et. al[3] and centering of the nanodiffraction patterns. Next, the variance $V(k)$ of the diffraction data was calculated as[4]

$$V(\mathbf{k}) = \frac{\langle I^2(\mathbf{k}, r)\rangle - \langle I(\mathbf{k}, r)\rangle^2}{\langle I(\mathbf{k}, r)\rangle^2}, \quad (1)$$

Where I is image intensity, $\mathbf{k}$ is the scattering vector, and $r$ is the position on the sample. After computing variance curves for each of the spatial locations shown in Figure S1(b), the curves were average to obtain a representative curve for the sample.

## II. XAS EXPERIMENTS

XAS measurements of the three oxidized niobium samples with the history described in Table 1 in the main text were carried out at O K-edge at beamline 4.0.2 of the Advanced Light Source (ALS), at Lawrence Berkeley National Laboratory, USA. The sample preparation is also described in the Table – no further treatments of the surface or sample were performed for the XAS measurements. The total electron yield detection technique was used during the XAS measurements.

In Figure S2, we plot the full XAS measurement data. In (a), we show the energy range relevant to the Nb M-edges. We find that these spectra do not vary enough from sample to sample to provide any reliable conclusions regarding the changes in morphology and structure. Figure S2(b) contains the C K edge, which likely comes from the environment. Figure S2(c) is the O K edge, which is discussed in depth in the main text. We find more significant changes between the samples for the O K-edge, which justifies our choice in focusing on these spectra. There is precedence for using the O K edge over the Nb spectra, for example in Ref.,[5] where the authors correlate O K edge peak positions with changes in valence of the Nb atom, whereas the correlation is less obvious in the Nb spectra. These results agree with the observation that the Nb XAS of any of our samples is dominated by the bulk Nb metal signal, while the O K edge reports solely on the oxide, which makes the O K edge the most appropriate spectrum for analysis. In Figure S2(d), we show the high energy region, which contains the Si K-edge in Samples 2 and 3, as expected for patterned structures, which leave exposed Si surfaces.

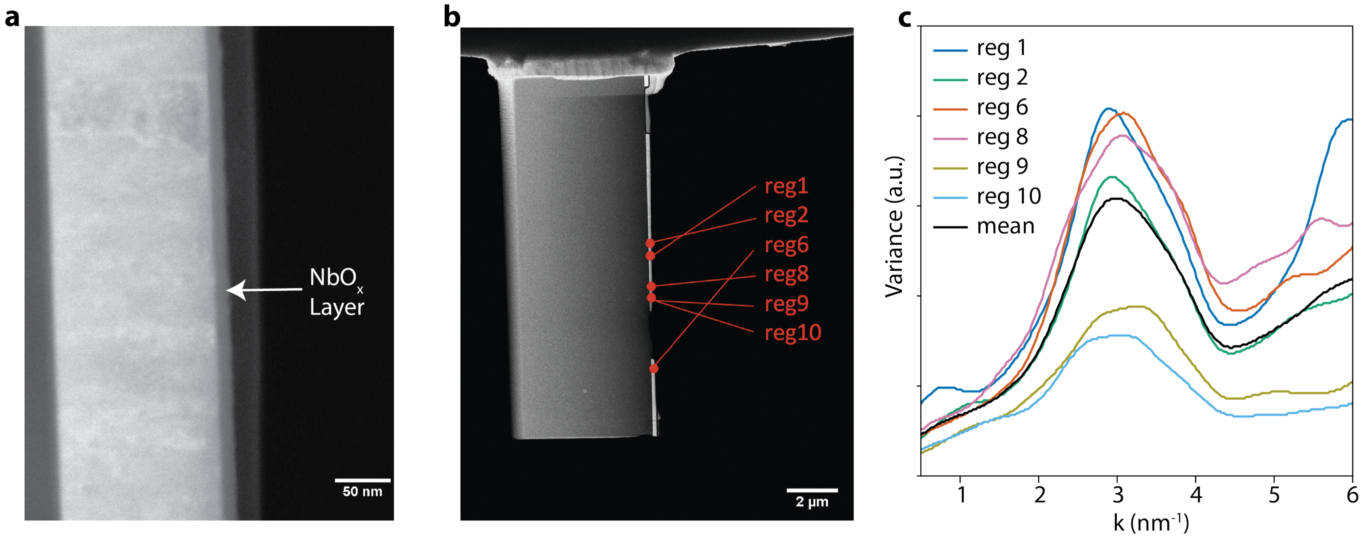


FIG. S1. (a) High-resolution TEM image of sample 2 cross-section used for FEM measurements. (b) Different regions of the Nb oxide film with varying thickness over which the electron microscope is used. (c) Spatial variance measuring the interatomic spacing between Nb centres in $Nb_2O_5$ obtained by radially integrating the FEM speckle pattern over the regions in (a).

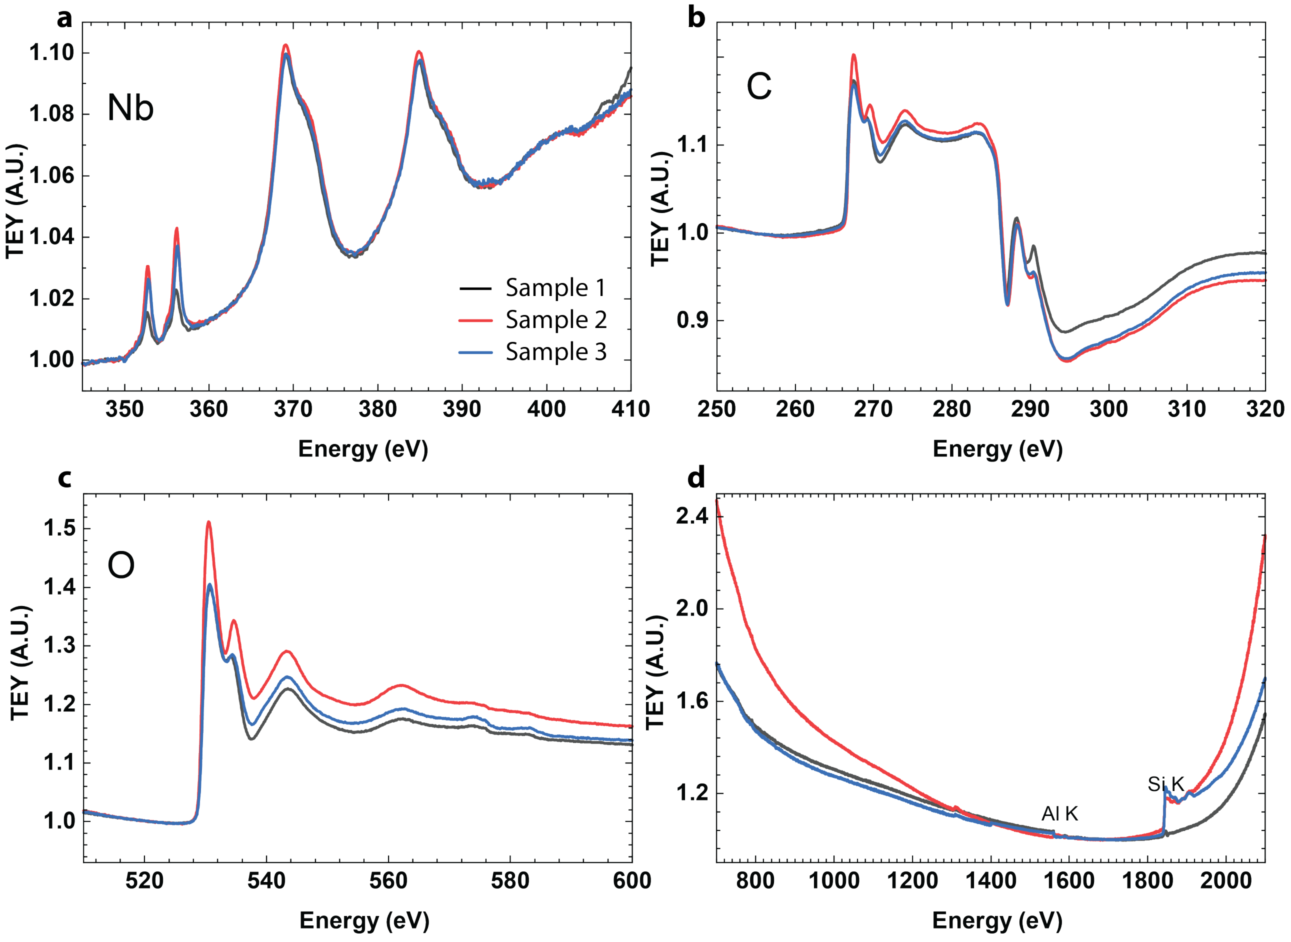


FIG. S2. Full XAS results for the (a) Nb M-edge, (b) C K-edge, (c) O K-edge, and (d) the high-energy ranges for Samples 1, 2 and 3 with treatments described in Table 1 in the main text.

### A. XAS Reference Spectra

We compared the measured XAS spectra to reference spectra from crystalline $NbO_2$, crystalline $Nb_2O_5$, and amorphous $SiO_2$ to find information about the oxidation state of the Nb atoms in our samples. The Nb oxide reference samples were powders purchased from Alfa-Aesar; product numbers 89692 and 11366 for $NbO_2$ and $Nb_2O_5$, respectively. We applied a 2.5 eV shift to align the dominant peak with previous experimental results,[6] which corrects any calibration errors in the XAS measurement. The $SiO_2$ reference is an amorphous layer of oxidized Si grown natively on a Si film. The oxidation state in our Nb oxide films can indicate the presence of unpaired $d$-electrons in the oxide layer. We compare Sample 1 (an unpatterned film) and the reference spectra in Figure S3(a). We find that none of the crystalline reference spectra can individually account for the observed features in the spectra of our samples. Also, we find that the $SiO_2$ reference spectrum contains a strong peak near 528 eV, which is completely absent from the spectra from each of our samples, suggesting $SiO_2$ is not present in large enough levels to be observed. It is possible that the 528 eV peak is the $\pi^*$ transition from adsorbed oxygen species (or other artifacts) on the reference sample, which may not be present in our samples. Therefore, we cannot completely rule out the possibility that there is some $SiO_2$ signal in our XAS, especially because there are exposed Si surfaces, seen in Figure S2d. However, we expect that the contribution to the total signal is small ($< 5\%$) because the ratio of exposed Si/Nb surfaces is known from the patterning procedure.

To investigate if a combination of reference spectra can explain the observed sample spectra, we perform a non-negative least-squares fit using the reference spectra as basis functions. Before performing the fit, we normalized each spectrum by subtracting the minimum value in the 520-560 eV energy window, and normalizing the maximum value of each spectrum to unity. We then smoothed the $NbO_2$ and $Nb_2O_5$ spectra using a moving average over a 1 eV window. After this, we fit the spectrum of Sample 1, shown in Figure S3(b), in which we clearly find that the resulting best fit does not match the observed spectrum for Sample 1. This suggests that analysis using standardized crystalline references is not suitable for our amorphous Nb-oxide films.

## III. DENSITY FUNCTIONAL THEORY CALCULATIONS

We applied a Hubbard-U of 4 eV to the Nb-$d$ states to account for the localization of these transition-metal orbitals, which is consistent with previous DFT+U studies on Nb-oxides.[7] The sensitivity of the calculated magnetic properties with our choice of U was studied in previous work,[8] where it was found that the projected magnetic moments slightly increase with the value of U, as expected. Furthermore, the calculated bandgaps of a variety of polymorphs of $Nb_2O_5$ compared reasonably well with experimental values for U=4 eV.

## IV. XAS CALCULATIONS

The structures of the amorphous phases were taken from Ref,[8] while those of the crystalline phases were taken from Inorganic Crystal Structure Database. An energy cut-off of 92 Ryd. was used in the DFT calculations, and a simplified Hubbard U of 4 eV was applied to the Nb $d$ orbitals. The 'O-high' and 'Nb-sp' pseudopotentials from PseudoDojo were used. For the BSE calculations, the electron orbitals were down-sampled onto real space grids chosen to match 1 grid point per 1 a.u., the k-point meshes were chosen to exceed 1 grid point per 0.16 a.u.$^{-1}$, and the number of conduction bands was set to 0.126 times the unit cell volume (in a.u.$^3$). For the screening, electron orbitals were calculated on k-point meshes exceeding 1 grid point per 0.56 a.u.$^{-1}$, and the number of conduction bands was set to 0.437 times the unit cell volume (in a.u.$^3$). A Lorentzian core-hole broadening of 0.07 eV was included, and additional Gaussian broadening of 0.5 eV was applied.

To compare the calculated spectra to the XAS sample spectra, all calculated spectra are stretched by a factor of 1.144 to correct for the known underestimation of band localization using semi-local density functionals. We did this by applying the stretching factor, and translating the spectrum back such that the position of the center of the dominant peak near 10 eV (in relative units) remained fixed. The optimization was performed using the LEAST_SQUARES package in SCIKIT-LEARN.[9]

## V. MACHINE LEARNING CORRELATIONS BETWEEN STRUCTURE AND SPECTRA

We next use principal component analysis and machine learning to identify correlations between the calculated and measured XAS spectra, and the presence of magnetic impurities in the samples. Our calculated XAS spectra in Figure 3 in the main text is the sum over all individual atomic XAS spectra in a given phase. Including each calculated phase, we have 1250 distinct XAS spectra, considering each individual atomic spectrum separately. Principal component analysis (PCA) was performed first on this set of 1250 atomic XAS calculations for the a window from 4.6 eV to 15.4 eV (on the relative scale of the calculations). We find that from the cumulative explained variance ratio in Figure S5(a) that 99.99 % of the variance of the spectral features can be explained by just 15 components. The compression of information is possible because the calculated spectra are highly correlated with one another; each individual spectrum is smooth with no random scatter. With these 15 principal components, the 1250 atomic spectra are projected onto the principal components to construct the latent space.

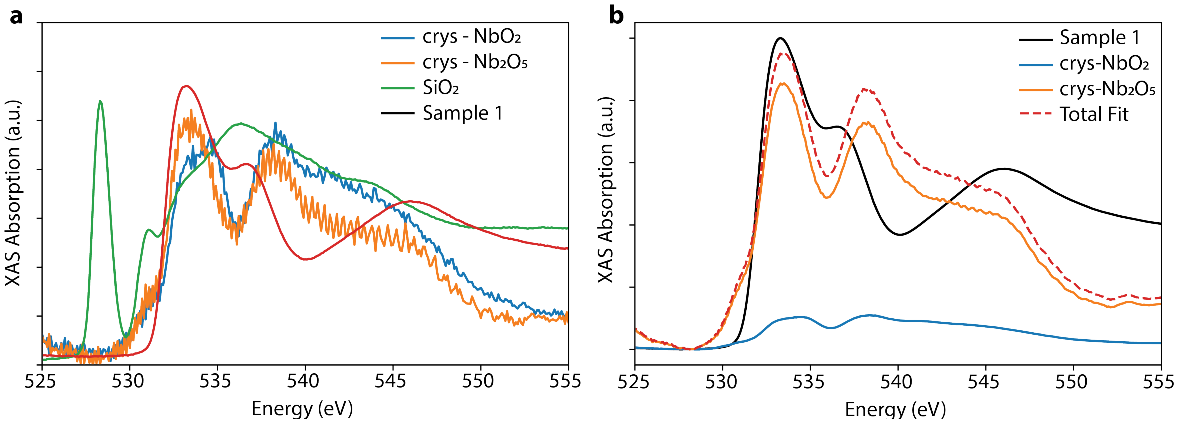


FIG. S3. (a) Comparison of each reference XAS spectrum to Sample 1 spectrum. (b) Non-negative best fit of a linear combination of reference spectra fit to the Sample 1 spectrum. The $SiO_2$ signal was not included in the fit because of the presence of several spectral features that clearly do not represent the measured data of the amorphous film. The c-$Nb_2O_5$ and c-$NbO_2$ signals were smoothed by calculating a moving average over a 1 eV window.

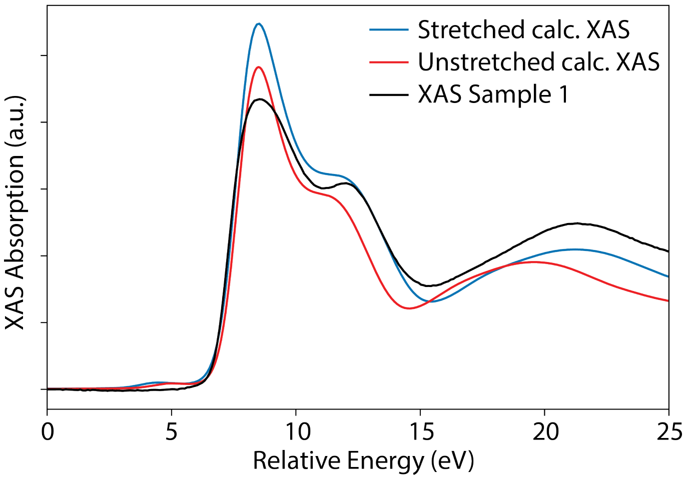


FIG. S4. Comparison of stretched and unstretched average amorphous XAS calculations to the Sample 1 spectrum.

After projection of the calculated XAS spectra onto this latent space, we calculate the structural descriptors for each O atom using similar methods to those used previously.[8] The main difference between the descriptors constructed in this work and the previous is that nearest neighbor versions of each descriptor are also calculated, excluding nearest neighbor versions of the Voronoi indices. Since there are multiple nearest neighbors in general, the descriptors are calculated for each neighbor, and averaged to create the final descriptors.

With the set of 1250 distinct spectra, we calculate the spectral variance of our XAS results, shown in Figure S6(b). Despite the lack of spectral features near 6 eV in the average calculated spectrum, we observe a large variation. To correlate changes in magnetic moment with XAS spectra, we label each atomic XAS spectrum with the magnetic moment on the oxygen atom, and the maximum moment on the nearest neighbor Nb atoms. We construct the covariance matrix between the spectral values at each energy bin and magnetic moments, and take the components of the matrix associated with $p$- and $d$-type magnetic impurities (magnetic moments on the O atom and on the Nb atoms, respectively), which defines the degree of variation expected with a change in magnetic moment. We can plot the expected changes to the spectrum via,

$$S_{d/p}(E) = \mu_S(E) + \sigma_{d/p,S}\Delta_{d/p}, \qquad (2)$$

in which $S(E)$ is the spectrum as a function of energy, the label $d/p$ specifies the type of magnetic impurity, $\mu_S$ is the average calculated spectral values, $\Delta_{d/p}$ is the change in the magnetic moment, and $\sigma_{d/p,S}$ is the covariance between spectral changes and magnetic impurities. We plot the expected spectrum for a $d$-type and $p$-type magnetic impurity in Figure S6a assuming a value of 1 for both $\Delta_d$ and $\Delta_p$, which correspond to a typical value for localized magnetic moments observed in our calculations. We find that the $p$-type magnetic impurity spectra have a strong feature at $\approx 6$ eV, which is indicative of the mid-gap magnetic impurity state described elsewhere.[8] The $d$-type impurity spectrum is very similar to the average spectrum, with an increased splitting between the two dominant peaks indicating an increased crystal field splitting. From the covariance matrix, we find that this increase in crystal field splitting is correlated with increases in bond lengths and nearest neighbor volumes, which are good indicators of the presence of a magnetic impurity since electron doping decreases the local charge of a Nb atom, repelling neighboring oxygens.

The variances of the calculated spectra describe which portions of the experimental spectra can be explained by our calculated data. For the three sample measurements, we define a window between 4 eV and 16 eV (on a relative scale) in which our calculations adequately describe the experimental spectra (vertical dashed lines in Figure S6b). The features in the experimental spectra out-

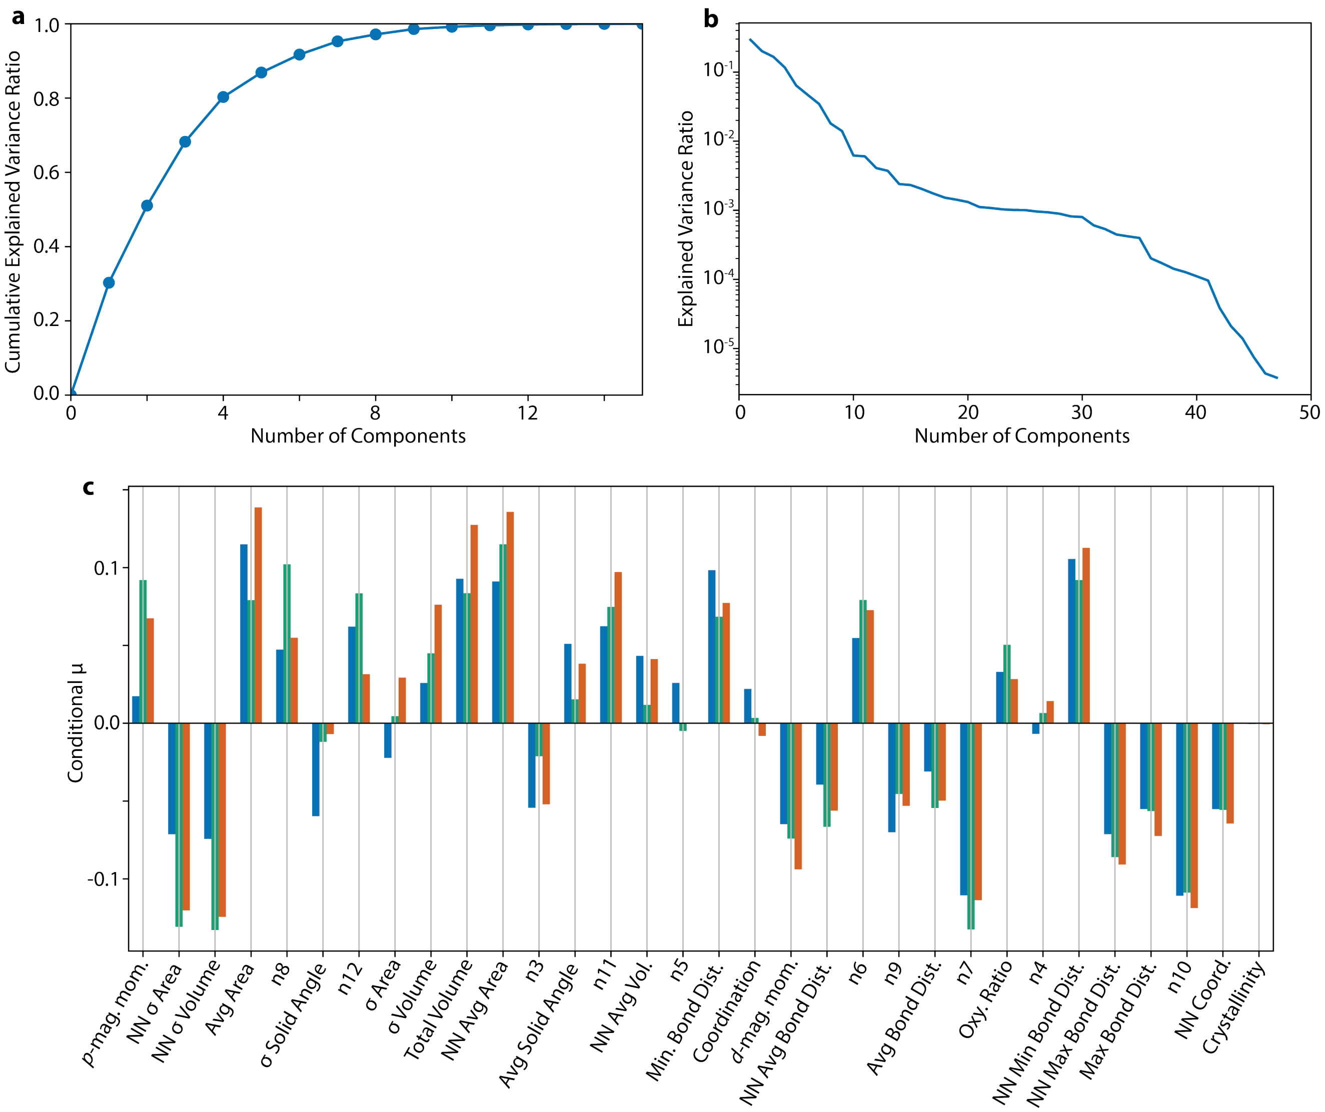


FIG. S5. (a) Cumulative explained variance ratio for principal component analysis (PCA) of calculated XAS spectra. (b) Scree plot for explained variance ratio for PCA of latent spectral features (determined from part (a)) and structural descriptors. (c) Full plot of conditional mean for each structural descriptor calculated given the three sample spectra.

side of this energy window can not be reliably described by our calculations as the experimental spectra are more than one standard deviation away from the average calculated spectrum. This means that the experimental spectra in these regions are primarily described by outliers in our calculated data, which do not provide good enough statistics to draw confident conclusions from the data. Additionally, it is difficult to get proper absorption over a broad range for soft x-rays with self-absorption effects, so it is important to limit the scope of our analysis to a reliable range.

As the features of an XAS spectrum are strongly determined by local structure and morphology, we seek to find correlations between structural descriptors and calculated XAS spectra using machine learning. The structural descriptors used for this analysis were chosen to maximize the ease of interpretation of the final results. The structural descriptors can be partitioned into four groups: (1) bond length statistics, (2) coordination numbers, (3) polyhedra shape type, and (4) polyhedra geometry statistics. The statistics calculated mean and standard deviation, but the bond length statistics also included the minimum and maximum bond lengths as these were found to be important in determining the presence of magnetic impurities in amorphous $NbO_x$ materials.[8] We defined our polyhedra using the Voronoi polyhedra description, which are constructed from planes between the central atom and its nearest neighbors. Since each XAS spectrum provides information on the atom itself and its nearest neighbors, we created two versions of each of these descriptor groups; one based on the O atoms themselves, and another for the nearest neighbor

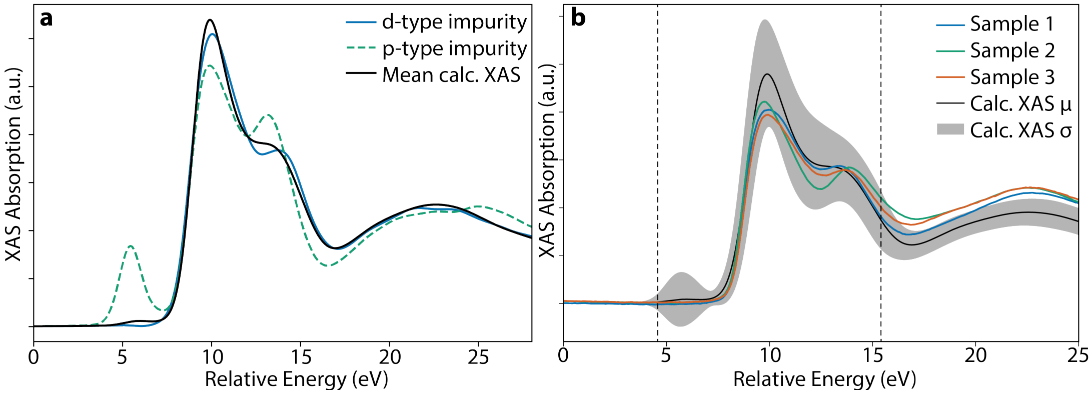


FIG. S6. (a) Expectation of the XAS spectrum based on the conditional information that the $d$- or $p$-type impurity density is 1. In this plot we also show the average calculated spectrum for comparison. (b) We compare the three experimental spectra to the average calculated spectrum with one standard deviation of spectral variance represented as grey shading. The vertical dashed lines represent the region in which the information in the calculated spectra can reliably explain the changes in the three experimental spectra.

Nb atoms associated with each O atom.

We next compress the 950 spectral components onto the 15 component latent space, described above. Then, we concatenate this dataset with the calculated structural descriptors, yielding a 47 component (32 structural descriptors plus 15 latent spectral features) dataset of 1250 samples. After this, we perform PCA again on the new dataset. To analyze which structural descriptors most correlate with changes in XAS spectra, we construct the covariance matrix from the PCA results, and contract the matrix in the following way:

$$c_i = \sum_j |\sigma_{ij}^{SL}| \tag{3}$$

$$\boldsymbol{\sigma} = \begin{pmatrix} \boldsymbol{\sigma}_{SS} & \boldsymbol{\sigma}_{SL} \\ \boldsymbol{\sigma}_{LS} & \boldsymbol{\sigma}_{LL} \end{pmatrix} \tag{4}$$

in which $\boldsymbol{\sigma}$ is the full covariance matrix, $\boldsymbol{\sigma}^{SS}$ is the block pertaining to the structural descriptors, $\boldsymbol{\sigma}^{SS}$ pertains to the latent spectral features, $\boldsymbol{\sigma}^{SL}$ is the covariances between the structural and latent features, and $c_j$ is a covariance metric describing the degree to which a structural descriptor $j$ is covariant with the spectral features. Figure S7 shows which structural descriptors have the largest covariances with XAS spectra. We find that the $p$-type magnetic impurity density is most covariant with an O K-edge XAS spectrum. The remaining highly covariant features are a mix of structural features attributed to either nearest neighbor (NN) or the O atom itself, indicating that changes in XAS spectra do signify changes in structural characteristics. This analysis helps explicitly describe the types of information present in XAS spectra of amorphous Nb oxides.

To determine the types of structural changes in the three experimental XAS spectra, we calculate the conditional mean of each structural descriptor given the values of the experimental spectrum projected onto the latent

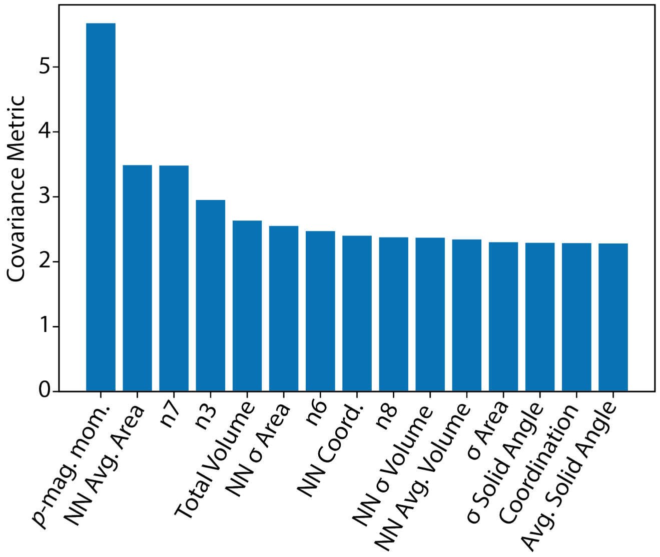


FIG. S7. (a) Covariance metric (defined in text) describing the amount of variation of a given structural descriptor with changes in the XAS spectrum. Larger covariances describe descriptors that are more easily studied with XAS.

space. The conditional means were calculated via,

$$\boldsymbol{\mu}_{S|\mathbf{x}_L} = \boldsymbol{\mu}_S + \boldsymbol{\sigma}_{SL} \cdot \boldsymbol{\sigma}_{LL}^{-1} \cdot (\mathbf{x}_L - \boldsymbol{\mu}_L) \tag{5}$$

where $\boldsymbol{\mu}_{S/L}$ is the mean of the structural or latent spectral feature, $\mathbf{x}_L$ is the value of a provided experimental spectrum projected onto the latent variables, and the $\boldsymbol{\sigma}$ blocks are defined above. Eq. 5 is defined in the most general way, but in practice, we pre-process the data to set the means and variances of each feature to zero and one, respectively, simplifying the equation.

After calculating the conditional mean for each experimental spectrum, we sort the data by the ascending relative feature variation between the three Samples, shown

| Feature | Sample 1 | Sample 2 | Sample 3 |
|---|---|---|---|
| $p$-type mag. mom. | 0.0062 | 0.0095 | 0.0084 |
| $d$-type mag. mom. | 0.0149 | 0.0140 | 0.0122 |

TABLE I. Expected magnetic moment per O/Nb atom for $p$- and $d$-type impurities, respectively.

in Figure S5(c). Each of these conditional means are expressed in a normalized basis, that is, each value is normalized by its sample standard deviation. We find that the $p$-type impurity density is predicted to be larger in the experiments than what we find in our calculations. We also find that the shape characteristics are changed, with lower variance in the NN polyhedron area and volume, indicating some more structural order in the experiments compared to the calculations. Also, the average polyhedron volumes for both Nb and O atoms are expected to be larger in the experiments relative to the calculations, leading to larger minimum bond distances, which correlates with larger $p$-type moments that typically need more physical space to accommodate an extra electron. We also find that the $d$-type magnetic impurity density is reduced relative to the average value observed in our calculations

Comparing the differences between the experimental values, we find that qubit chip sample (with an oxide thickness of 15 nm) is predicted to have the largest $p$-type impurity densities, and the unpatterned film is predicted to have the largest $d$-type impurity density. Also, the polyhedron variances of the Nb atoms are increased in the unpatterned Nb-oxide film (Sample 1), indicating that the fabrication treatments, such as heating to $\sim 150°$C in resist removal, tend to favor local structural order in oxide films. Conversely, we find that the polyhedron variances on the O atoms are reduced in the unpatterned film, which suggests the presence of voids nearest to the O atoms in the patterned films.

To most quantitatively explain the expected variation of the $p$- and $d$-type magnetic impurities associated with each sample, we remove the normalization for each magnetic conditional mean as shown in Table I. For $p$-type magnetic impurities, we find that Sample 2, the qubit chip with the thickest oxide layer, has the highest expected density of magnetic impurities, and Sample 1 has the highest $d$-type impurity density, but the differences are small. All samples have elevated $d$-type impurities relative to $p$-type impurities, which is more detrimental to resonator quality factor.[8,10] Comparing the patterned films, the resonator chip has lower magnetic impurity densities, regardless of type of impurity. This is likely caused by the additional fabrication steps in producing a qubit chip (patterning of Josephson junctions, annealing, etc.). We express these values in a Bohr magneton per mole basis; in which we observe that there are $1.79 \times 10^{22}$, $1.69 \times 10^{22}$, and $1.46 \times 10^{22}$ $\mu_B$ of $d$-type impurities per mole of $Nb_2O_5$ for Samples 1, 2, and 3 respectively for better comparison with experiments.

**Disclaimer** Specific software and hardware is identified for information purposes only and is not intended to imply recommendation or endorsement by NIST.

[1] E. Kennedy, N. Reynolds, L. Rangel DaCosta, F. Hellman, C. Ophus, and M. Scott, "Tilted fluctuation electron microscopy," Applied Physics Letters **117**, 091903 (2020).
[2] J. Hwang and P. Voyles, "Variable resolution fluctuation electron microscopy on cu-zr metallic glass using a wide range of coherent stem probe size," Microscopy and Microanalysis **17**, 67–74 (2011).
[3] C. Gammer, C. Ophus, T. C. Pekin, J. Eckert, and A. M. Minor, "Local nanoscale strain mapping of a metallic glass during in situ testing," 10.1063/1.5025686.
[4] M. Treacy, J. Gibson, and P. Keblinski, "Paracrystallites found in evaporated amorphous tetrahedral semiconductors," Journal of Non-Crystalline Solids **231**, 99–110 (1998).
[5] R. Tao, R. Todorovic, J. Liu, R. J. Meyer, A. Arnold, W. Walkosz, P. Zapol, A. Romanenko, L. D. Cooley, and R. F. Klie, "Electron energy-loss spectroscopy study of metallic nb and nb oxides," J. Appl. Phys. **110**, 124313 (2011).
[6] M. J. Olszta, J. Wang, and E. C. Dickey, "Stoichiometry and valence measurements of niobium oxides using electron energy-loss spectroscopy," Journal of Microscopy **224**, 233–241 (2006).
[7] C. P. Koçer, K. J. Griffith, C. P. Grey, and A. J. Morris, "First-principles study of localized and delocalized electronic states in crystallographic shear phases of niobium oxide," Physical Review B **99**, 075151 (2019).
[8] E. Sheridan, T. F. Harrelson, E. Sivonxay, K. A. Persson, M. V. P. Altoe, I. Siddiqi, D. F. Ogletree, D. I. Santiago, and S. M. Griffin, "Microscopic theory of magnetic Disorder-Induced decoherence in superconducting nb films," (2021).
[9] F. Pedregosa, G. Varoquaux, A. Gramfort, V. Michel, B. Thirion, O. Grisel, M. Blondel, P. Prettenhofer, R. Weiss, V. Dubourg, J. Vanderplas, A. Passos, D. Cournapeau, M. Brucher, M. Perrot, and E. Duchesnay, "Scikit-learn: Machine learning in Python," Journal of Machine Learning Research **12**, 2825–2830 (2011).
[10] J. Halbritter, "On the oxidation and on the superconductivity of niobium," Applied Physics A Solids and Surfaces **43**, 1–28 (1987).
